# Supplementary material for: Few-shot Image Generation Using Discrete Content Representation
Source: arXiv:2207.10833 source file (2022-07-22)
Supplement: Supplementary file 5 [file visualization_supple_1st_stage.tex]

\begin{figure*}
\begin{center}
\includegraphics[scale=0.51]{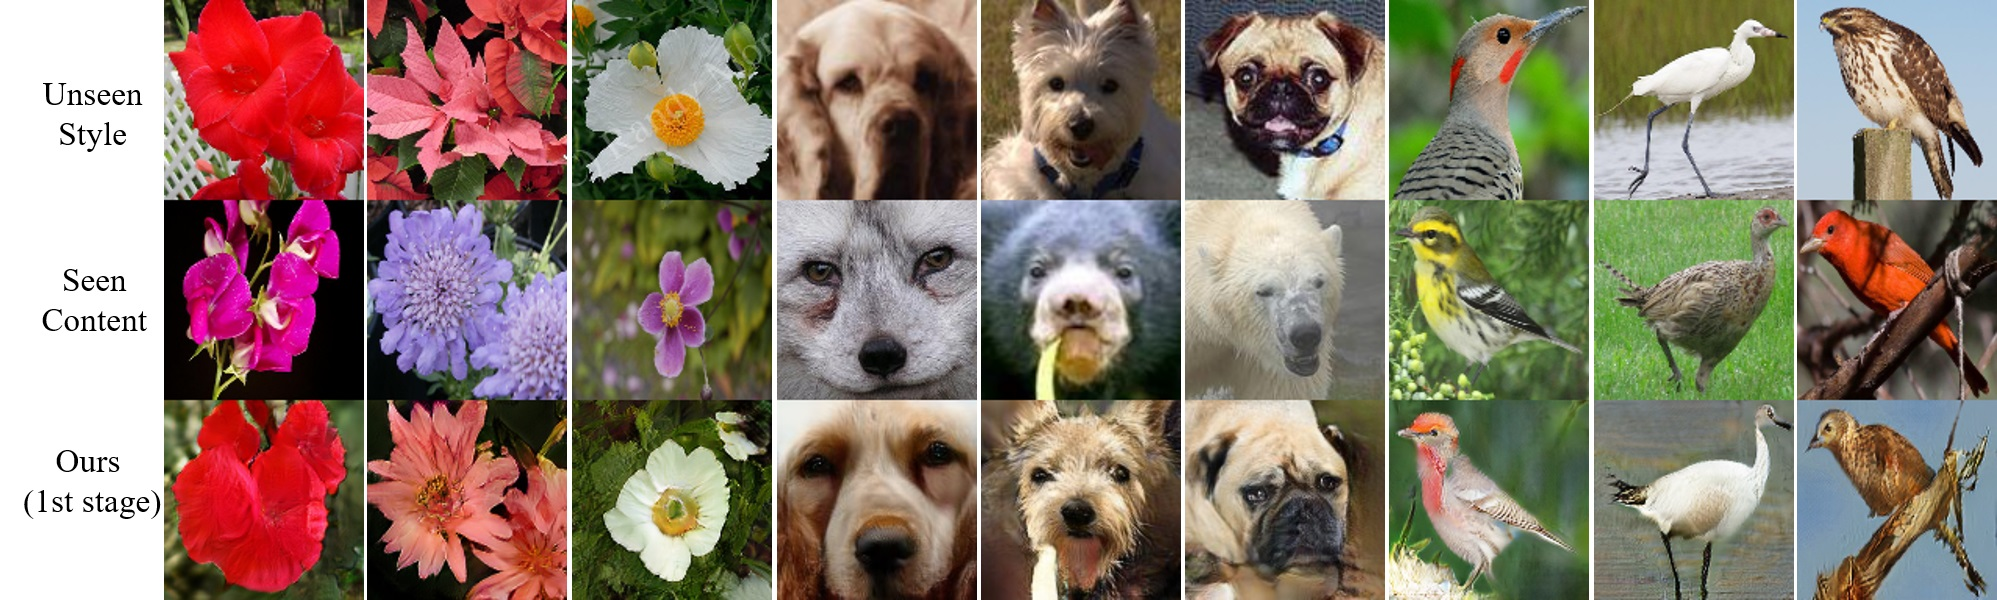}
\end{center}
\caption{Images generated by FUNIT, COCO-FUNIT, and Disco-FUNIT(1st stage) in 1-shot setting on Flowers, Animal Faces, and NABirds dataset. (from top to bottom: unseen style images, seen content images, images generated by Disco-FUNIT (1st stage)).}
\label{fig:more_images_1stage} 
\end{figure*}
